# Supplementary material for: Automated Code generation for Information Technology Tasks in YAML through Large Language Models
Source: arXiv:2305.02783 source file (2023-05-23)
Supplement: Supplementary file 1 [file appendix.tex]

% \section*{More Details on Dataset}
% \begin{table*}
% \centering
% \begin{tabular}{|l|p{9cm}|}
% \hline
% \textbf{Key} & \textbf{Description}\\
% \hline
% repo\_name & name of the repository (or Ansible Galaxy namespace) this sample belongs to \\
% \hline
% repo\_id & id of the repo (or Ansible Galaxy role/collection) this sample belongs to \\
% \hline
% text & content of the target YAML sample \\
% \hline
% type & indicator of what this sample YAML represents-- a task or a playbook\\
% \hline
% metadata & other relevant information pertaining to this sample, e.g. `role', `collection', repo\_branch %\\
% \hline
% path & location of the file within the repo corresponding to this sample  \\
% \hline
% source & source of the dataset from which this sample was extracted, e.g., ansible galaxy, github, %gitlab, etc.\\
% \hline
% license & OSS License\\
% \hline
% \end{tabular}
% \caption{Dataset Schema} 
% \label{table-dataset-schema}
% \end{table*}

% \subsection*{Data collection for Fine-tuning Datasets}
% %\todo{Move this to sec Generation types}}
% In order to create the dataset we start with a file from Ansible Galaxy.
% If the file is a playbook, we check if it contains one or more playbooks.
% We consider each playbook individually.
% If the playbook contains one or 2 tasks, we consider it to be a Type 1 sample.
% If it contains more tasks, we use it to create multiple Type 4 samples.
% The Role file from Ansible Galaxy is similarly used to create one Type 2 sample with the first task and multiple Type 3 samples with at least one task in the input context.
% We ignore all tasks and playbooks which do not contain the ``- name'' field, since we need this field to extract the prompt.
% Syntax check is used to ensure we only consider valid Ansible, YAML samples.

% Table~\ref{table-dataset-schema} shows the information extracted and stored with each YAML sample in the dataset.
